# Supplementary material for: Safe Reinforcement Learning via Curriculum Induction
Source: arXiv:2006.12136 source file (2021-01-21)
Supplement: Supplementary file 1 [file related_work.tex]

\section{Related Work}\label{sec:app:RelatedWork}

\andrey{For now, just dumping here the related work content that used to be in the intro. We should expand (e.g., describing more of CMPD literature here, and cite \citep{le2019batch}) and potentially move it elsewhere.}

The problems of improving RL's sample efficiency using a curriculum and of making RL safe have been studied extensively but in isolation from each other. \citet{narvekar2016source} proposes a library of standardized ways of modifying an RL environment to create a curriculum but does not investigate how to choose and when to propose subtasks to students. \citet{sukhbaatar2017intrinsic}'s approach repeatedly uses a copy of the student itself to generate a sequence of surrogate goals, trying to attain which makes the student learn faster. \citet{asada1996purposive} and \citet{florensa2017reverse} build a curriculum by modifying the agent's initial state distribution, \citet{florensa2017automatic} does so via automatic goal-setting, \citet{riedmiller2018learning} -- by modifying the reward function, and \citet{wu2016training} -- by changing the dynamics. Some curriculum learning approaches make explicit use of environment parameterization when constructing a curriculum \citep{portelas2019cts,wang2019poet}. While curriculum learning can increase the efficiency of RL or help it converge to a high-quality policy, by itself it does little to make learning safe. To analyze RL safety, many works, including ours, rely on the constrained MDP (CMDP) formalism \citep{altman1999constrained}. Some existing RL algorithms that make safety a priority take heuristic approaches to achieving it \citep{achiam2017constrained}. Others use the control-theoretic notion of Lyapunov functions to maintain safety if the agent is initialized with a safe policy \citep{chow2019lyapunov} or to guarantee it after the agent has discovered a safe policy during learning \citep{chow2018lyapunov}. In order to make sure that the agent can safely explore during RL, \citet{berkenkamp2017safe} make smoothness assumptions about the functions that characterize safety of various states. Yet different techniques ensure that agent policies considered throughout learning satisfy conservative properties that imply safety \citep{el2016convex}. In general, safety guarantees in RL are attained with little regard to sample efficiency of the resulting algorithm and at the cost of making assumptions that are not easy to interpret, satisfy, and verify in many practical settings. The novelty of our work is in employing curriculum induction to make an RL agent learn faster while providing an intuitive, easy to understand characterization of the learning process safety.
